# Supplementary material for: Side-Channel Hardware Trojan for Provably-Secure SCA-Protected Implementations
Source: arXiv:1910.00737 source file (2019-09-22)
Supplement: Supplementary file 1 [file appendix.tex]

%\newpage
%\vspace{10mm}
\section{Uniform TI of $\mathcal{F}$}
\label{app:TI_F}
Considering $\mathbfit{y}=\mathcal{F}(\mathbfit{x})$ and $\mathbfit{x}^{i\in\{1,2,3\}}=\langle d^i,c^i,b^i,a^i\rangle$ -- derived by direct sharing -- we present one of its uniform sharing $\left(\mathbfit{y}^1,\mathbfit{y}^2,\mathbfit{y}^3\right)=$ $\left(\mathcal{F}^1\left(\mathbfit{x}^2,\mathbfit{x}^3\right),\mathcal{F}^2\left(\mathbfit{x}^3,\mathbfit{x}^1\right),\mathcal{F}^3\left(\mathbfit{x}^1,\mathbfit{x}^2\right)\right)$ as
\begin{align*}
	y^1_0 & = b^2 \oplus c^2a^2 \oplus c^2a^3 \oplus c^3a^2,\\
	y^1_1 & = c^2 \oplus b^2 \oplus d^2a^2 \oplus d^2a^3 \oplus d^3a^2,\\
	y^1_2 & = d^2 \oplus b^2a^2 \oplus b^2a^3 \oplus b^3a^2,\\
	y^1_3 & = c^2 \oplus b^2 \oplus a^2 \oplus d^2a^2 \oplus d^2a^3 \oplus d^3a^2,
\end{align*}
\begin{align*}	y^2_0 & = b^3 \oplus c^3a^3 \oplus c^1a^3 \oplus c^3a^1,\\
	y^2_1 & = c^3 \oplus b^3 \oplus d^3a^3 \oplus d^1a^3 \oplus d^3a^1,\\
	y^2_2 & = d^3 \oplus b^3a^3 \oplus b^1a^3 \oplus b^3a^1,\\
	y^2_3 & = c^3 \oplus b^3 \oplus a^3 \oplus d^3a^3 \oplus d^1a^3 \oplus d^3a^1,
\end{align*}
\begin{align*}
	y^3_0 & = b^1 \oplus c^1a^1 \oplus c^1a^2 \oplus c^2a^1,\\
	y^3_1 & = c^1 \oplus b^1 \oplus d^1a^1 \oplus d^1a^2 \oplus d^2a^1,\\
	y^3_2 & = d^1 \oplus b^1a^1 \oplus b^1a^2 \oplus b^2a^1,\\
	y^3_3 & = c^1 \oplus b^1 \oplus a^1 \oplus d^1a^1 \oplus d^1a^2 \oplus d^2a^1.
\end{align*}
